# Supplementary material for: CogBench: a large language model walks into a psychology lab
Source: arXiv:2402.18225 source file (2024-02-28)
Supplement: Supplementary file 1 [file llm_features.pdf]

| Model Name                    | No. of Parameters | Finetuned version of LLM | Use of RLHF | Open Source | Size of dataset | Context length | Conversational | Code |
|-------------------------------|-------------------|--------------------------|-------------|-------------|-----------------|----------------|----------------|------|
| gpt-4                         | 1760              | No                       | Yes         | No          | 1.56            | 8              | No             | No   |
| text-davinci-003              | 170               | No                       | Yes         | No          | 1.37            | 4              | No             | No   |
| text-davinci-002              | 170               | No                       | No          | No          | 1.37            | 4              | No             | No   |
| claude-1                      | 100               | No                       | RLAIF       | No          | 3.7             | 100            | No             | No   |
| claude-2                      | 200               | No                       | RLAIF       | No          | 7.4             | 100            | No             | No   |
| text-bison                    | 340               | No                       | Yes         | No          | 1.4             | 8              | No             | No   |
| falcon-40b                    | 40                | No                       | No          | Yes         | 0.54            | 2              | No             | No   |
| falcon-40b-instruct           | 40                | falcon-40b               | No          | Yes         | 0.6             | 2              | No             | No   |
| mpt-30b                       | 30                | No                       | No          | Yes         | 1.76            | 8              | No             | No   |
| mpt-30b-instruct              | 30                | mpt-30b                  | No          | Yes         | 1.8             | 8              | No             | No   |
| mpt-30b-chat                  | 30                | mpt-30b                  | No          | Yes         | 1.8             | 8              | Yes            | No   |
| llama-2-70                    | 70                | No                       | No          | Yes         | 2               | 4              | No             | No   |
| llama-2-13                    | 13                | No                       | No          | Yes         | 2               | 4              | No             | No   |
| llama-2-7                     | 7                 | No                       | No          | Yes         | 2               | 4              | No             | No   |
| llama-2-70-chat               | 70                | Yes                      | Yes         | Yes         | 2               | 4              | Yes            | No   |
| llama-2-13-chat               | 13                | Yes                      | Yes         | Yes         | 2               | 4              | Yes            | No   |
| llama-2-7-chat                | 7                 | Yes                      | Yes         | Yes         | 2               | 4              | Yes            | No   |
| vicuna-7b-v1.5                | 7                 | llama-2-7                | Yes         | Yes         | 2.37            | 4              | Yes            | No   |
| vicuna-13b-v1.5               | 13                | llama-2-13               | Yes         | Yes         | 2.37            | 4              | Yes            | No   |
| Llama-2-7b-longlora-100k-ft   | 7                 | llama-2-7                | No          | Yes         | 2               | 100            | No             | No   |
| Llama-2-7b-longlora-8k-ft     | 7                 | llama-2-7                | No          | Yes         | 2               | 8              | No             | No   |
| Llama-2-7b-longlora-16k-ft    | 7                 | llama-2-7                | No          | Yes         | 2               | 16             | No             | No   |
| Llama-2-7b-longlora-32k-ft    | 7                 | llama-2-7                | No          | Yes         | 2               | 32             | No             | No   |
| Llama-2-7b-longlora-32k       | 7                 | llama-2-7                | No          | Yes         | 2               | 32             | No             | No   |
| Llama-2-13b-longlora-32k-ft   | 13                | llama-2-13               | No          | Yes         | 2               | 32             | No             | No   |
| Llama-2-13b-longlora-64k      | 13                | llama-2-13               | No          | Yes         | 2               | 64             | No             | No   |
| Llama-2-13b-longlora-32k      | 13                | llama-2-13               | No          | Yes         | 2               | 32             | No             | No   |
| Llama-2-70b-longlora-32k      | 70                | llama-2-70               | No          | Yes         | 2               | 32             | No             | No   |
| Llama-2-70b-chat-longlora-32k | 70                | llama-2-70-chat          | Yes         | Yes         | 2               | 32             | Yes            | No   |
| LongAlpaca-7B                 | 7                 | llama-2-7                | No          | Yes         | 2               | 16             | Yes            | No   |
| LongAlpaca-13B                | 13                | llama-2-13               | No          | Yes         | 2               | 16             | Yes            | No   |
| LongAlpaca-70B                | 70                | llama-2-70               | No          | Yes         | 2               | 16             | Yes            | No   |
| CodeLlama-7B                  | 7                 | llama-2-7                | No          | Yes         | 2.5             | 16             | No             | Yes  |

|               |    |            |    |     |     |    |    |     |
|---------------|----|------------|----|-----|-----|----|----|-----|
| CodeLlama-13B | 13 | llama-2-13 | No | Yes | 2.5 | 16 | No | Yes |
| CodeLlama-34B | 34 | llama-2-34 | No | Yes | 2.5 | 16 | No | Yes |
